# Supplementary material for: Model of collective fish behavior with hydrodynamic interactions
Source: arXiv:1705.07821 source file (2018-05-03)
Supplement: Supplementary file 1 [file Supplemental_material.pdf]

# Supplementary Materials:
# Hydrodynamic interactions influence fish collective behavior

by Audrey Filella, François Nadal, Clément Sire, Eva Kanso, and Christophe Eloy

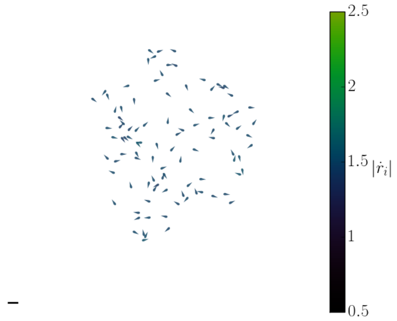


**Supplementary Movie 1.** Movie showing the swarming phase. Parameters are the same as in Fig. 2(a). The simulation last 25 dimensionless time units. The scale bar represents $10r_0$.

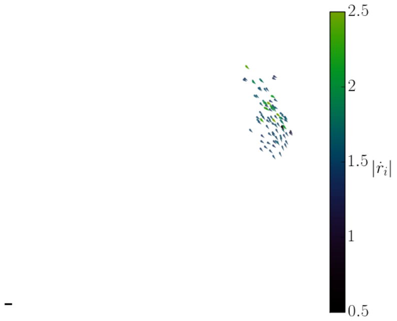


**Supplementary Movie 2.** Movie showing the schooling phase (Fig. 2b).

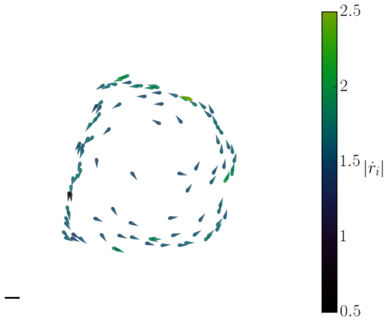


**Supplementary Movie 3.** Movie showing the milling phase (Fig. 2c).

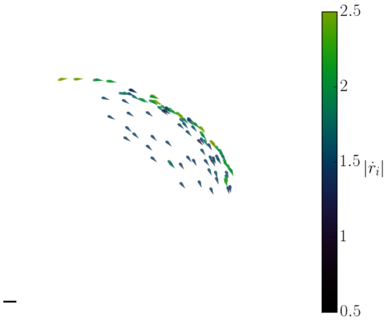


**Supplementary Movie 4.** Movie showing the turning phase (Fig. 2d).

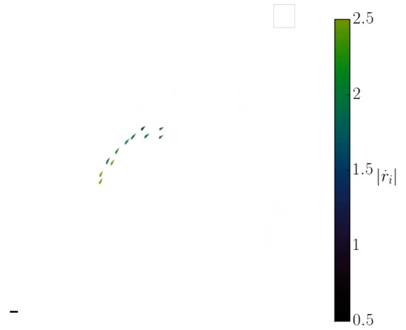


**Supplementary Movie 5.** Movie showing the turning phase for $N = 20$, $I_f = 10^{-2}$, $I_n = 0.1$, $I_{\|} = 0.4$.

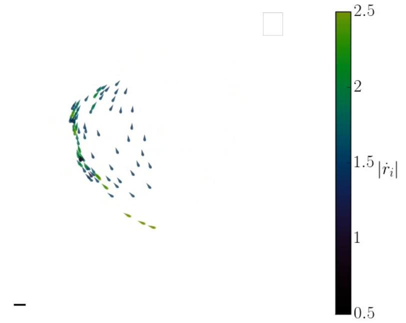


**Supplementary Movie 6.** Same as Supplementary Movie 5 for $N = 100$.

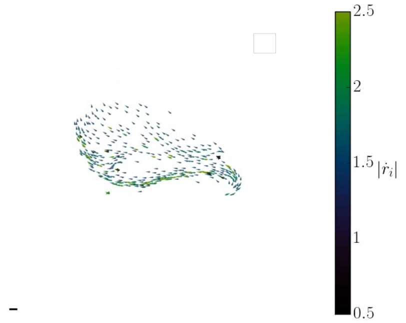


**Supplementary Movie 7.** Same as Supplementary Movie 5 for $N = 500$.

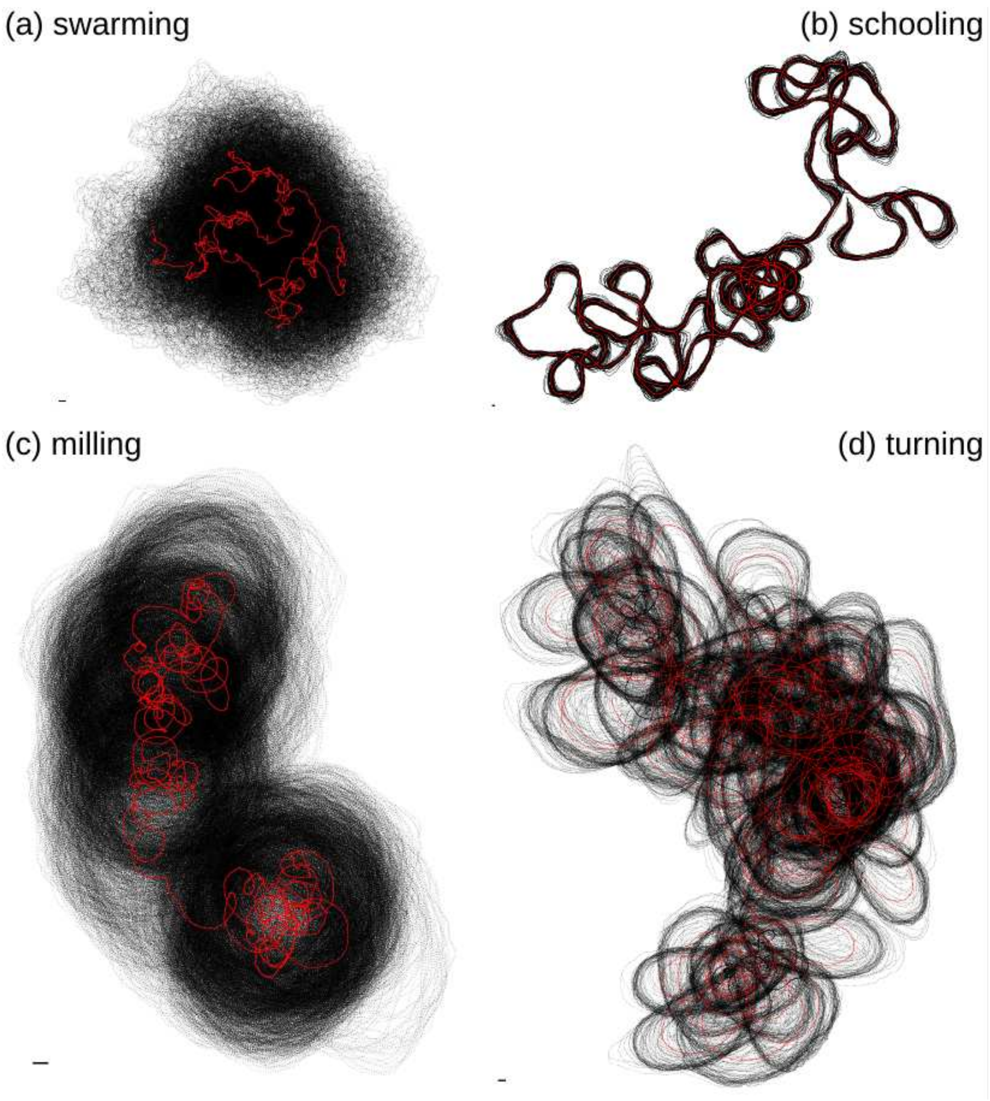


Supplementary Fig. 1: Trajectory of fish for each phase during 1900 dimensionless time units. Parameters are the same as in Figs. 2(a–d) of the Letter. Gray lines show the trajectory of individual fish and the red line show the trajectory of the center of mass. The scale bar corresponds to $10r_0$.

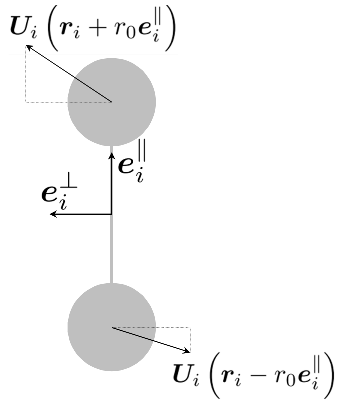


$$\Omega_i = \lim_{r_0\to 0} \frac{\boldsymbol{U}_i\left(\boldsymbol{r}_i + r_0\boldsymbol{e}_i^{\parallel}\right) - \boldsymbol{U}_i\left(\boldsymbol{r}_i - r_0\boldsymbol{e}_i^{\parallel}\right)}{2r_0} \cdot \boldsymbol{e}_i^{\perp} = \boldsymbol{e}_i^{\parallel} \cdot \nabla\boldsymbol{U}_i \cdot \boldsymbol{e}_i^{\perp}$$

Supplementary Fig. 2: Sketch of the swimmer seen as a dumbbell to explain the rotation term $\Omega_i$ used in the Letter [Eq. (5)]. Since we consider a potential and incompressible flow (*i.e.* $\boldsymbol{\nabla}\times\boldsymbol{u}_{ji} = \boldsymbol{\nabla}\cdot\boldsymbol{u}_{ji} = 0$ ), the calculation of $\Omega_i$ simplifies into $\Omega_i = \sum_{j\neq i} \partial_y u_{ji} \cos 2\theta_i - \partial_x u_{ji} \sin 2\theta_i$, where $u_{ji}$ is the $x$-component of $\boldsymbol{u}_{ji}$.

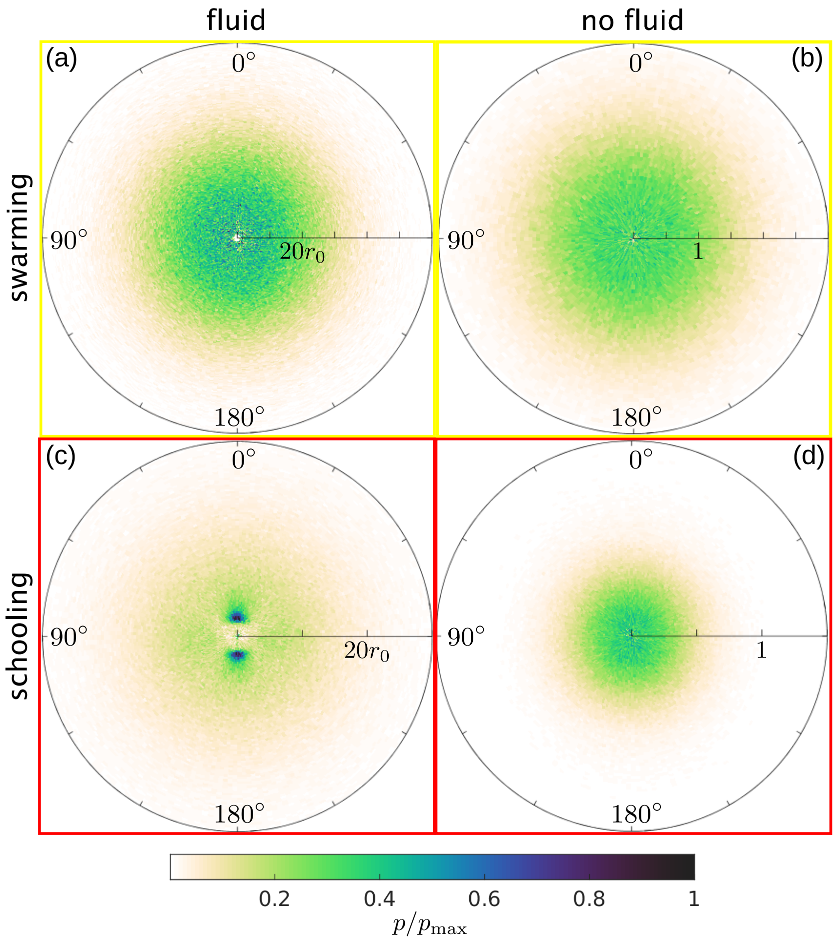


Supplementary Fig. 3: Heat maps showing the probability of presence $p(\rho, \theta)$ of the Voronoi neighbors in the framework of each individual. (a, c) Full hydrodynamic model, and (b, d) no fluid model. Top row is for swarming (a, b), bottom row is for schooling (c, d). The parameters are the same as the one used in Fig. 2a,b of the Letter.

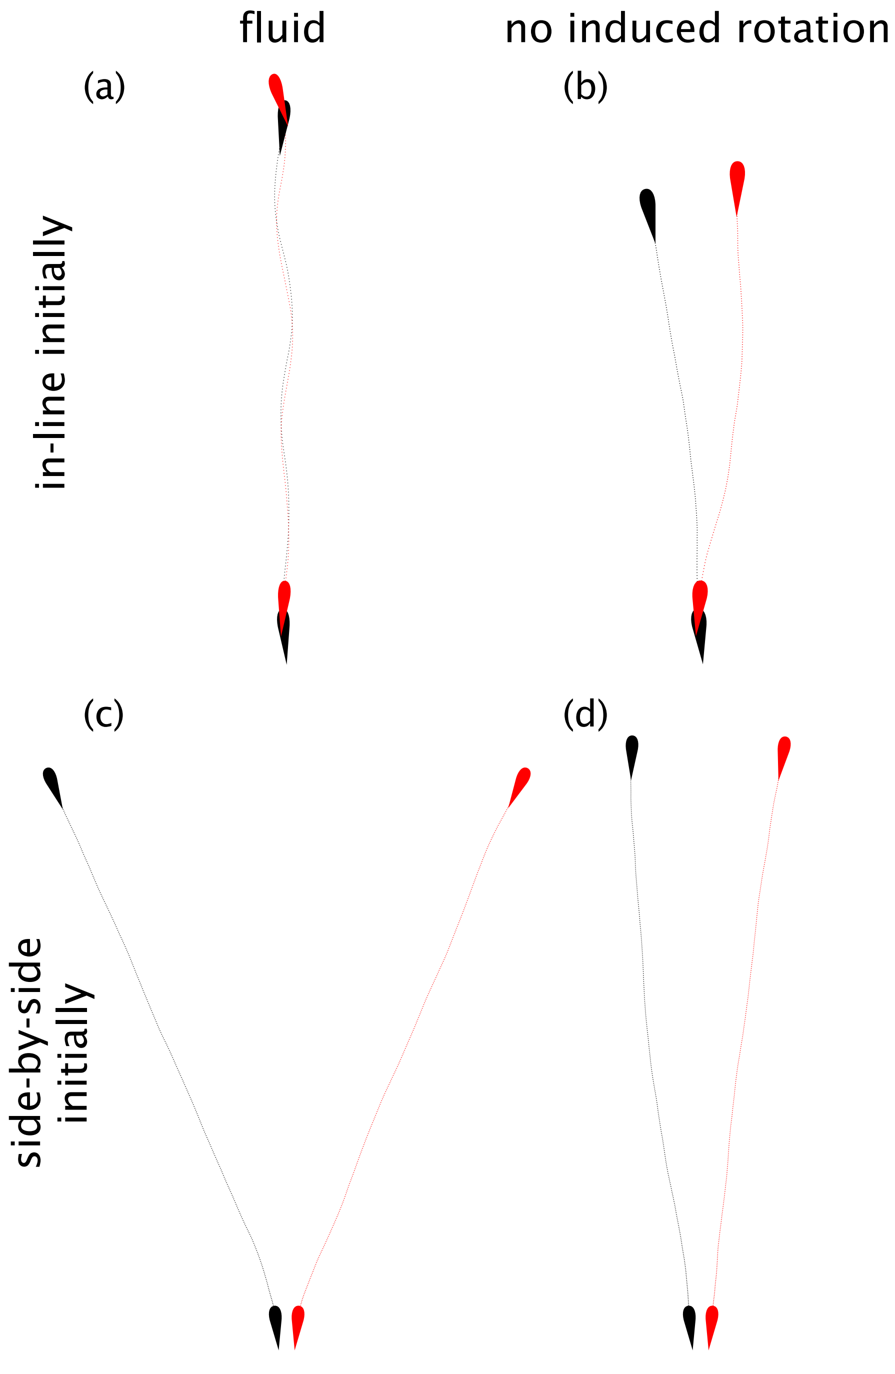


Supplementary Fig. 4: Dynamics of a fish pair with different initial condition and different fluid models, with no behavior (attraction and alignment have been set to zero). (a, b) Initially the two fish are in-line, (c, d) the fish are side-by-side. Left column shows the full hydrodynamic model (a, c), while the right columns (b, d) shows the dynamics with no induced rotation, i.e. $\Omega_i = 0$.

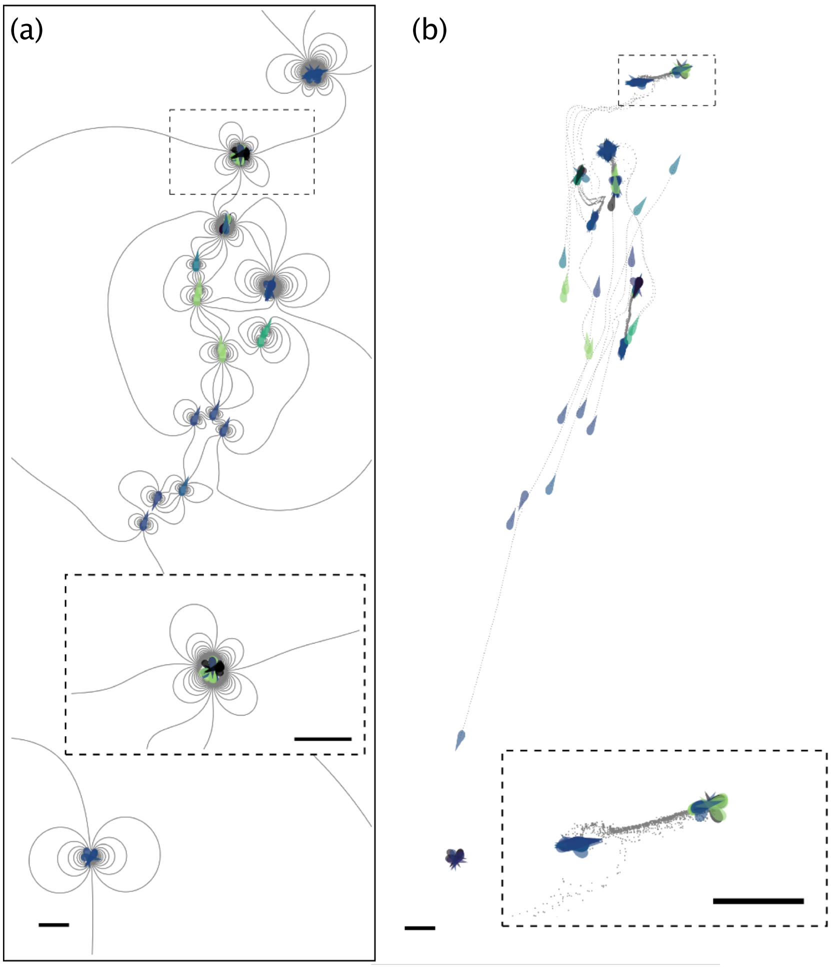


Supplementary Fig. 5: (a) Streamlines and positions of the fish when $I_n = 0$, $I_{\parallel} = 1$, and $I_f = 0.04$. Although the global order parameters are both small ($P = 0.11$, $M = 0.02$), this phase is very different from the swarming phase. Fish form clusters that move very slowly. (b) Two snapshots separated by 5 dimensionless time units (the second snapshot corresponds to a). The paths followed by each individual are shown in dotted lines.

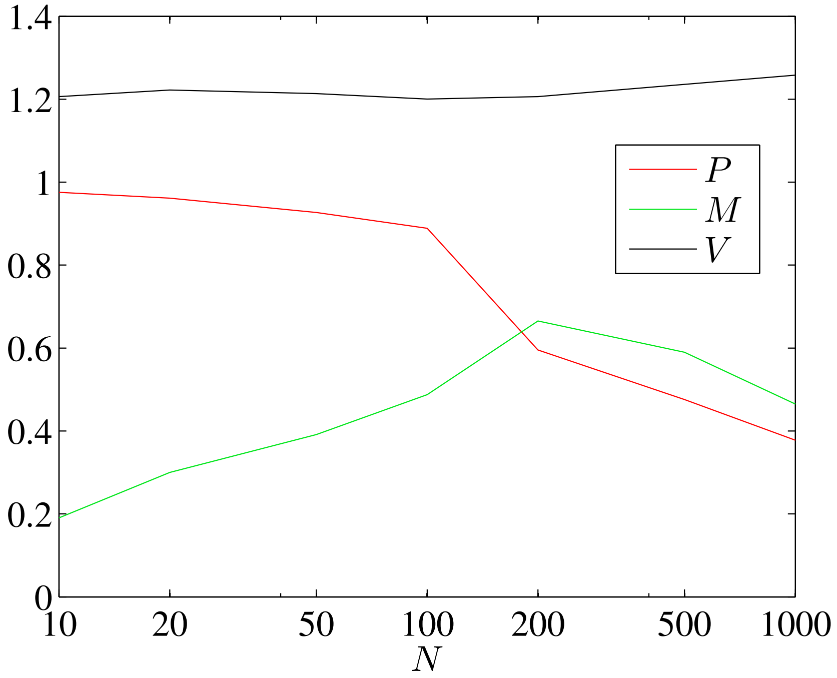


Supplementary Fig. 6: Values of the polarization $P$, milling $M$, and mean velocity $V$ when the number of swimmers $N$ is varied. The parameters are $I_f = 10^{-2}$, $I_n = 0.1$, $I_{\parallel} = 0.4$, such that the turning phase is observed for $N = 100$. As $N$ is increased, the angle of the circular sector covered by the population first increases up to $N = 200$ when $M$ is maximal and the dynamics resemble the milling phase. Then, for larger $N$ the turning becomes unstable and we observe alternatively dynamics that resemble turning and other that resemble milling, with sometimes a break-up into different subpopulations each following its own dynamics (see Supplementary Movies 5–7).

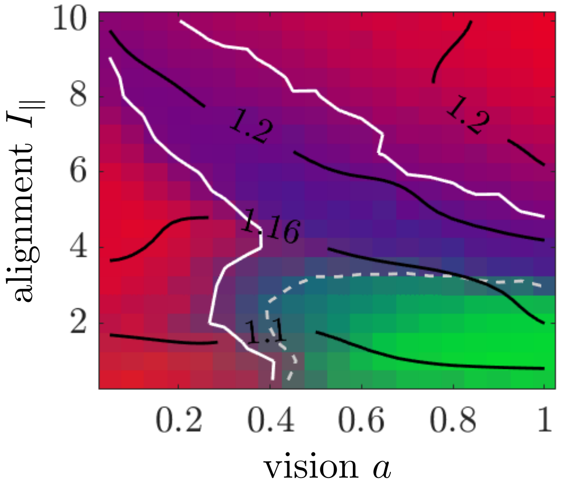


Supplementary Fig. 7: Phase diagram for $I_n = 0.1$, $I_f = 0.01$. Here the vision anisotropy $a$ is defined through the pre-factor $(1 + a\cos\theta_{ij})$ in Eq. 4 of the Letter. The anisotropy studied in the Letter corresponds to $a = 1$. This graph shows that, when $a$ tends to 0, the milling phase (green) disappears while the turning phase (purple) persists.
